# Supplementary material for: Measuring the dynamical evolution of the United States lobbying network
Source: arXiv:2503.11745 source file (2026-02-05)

A

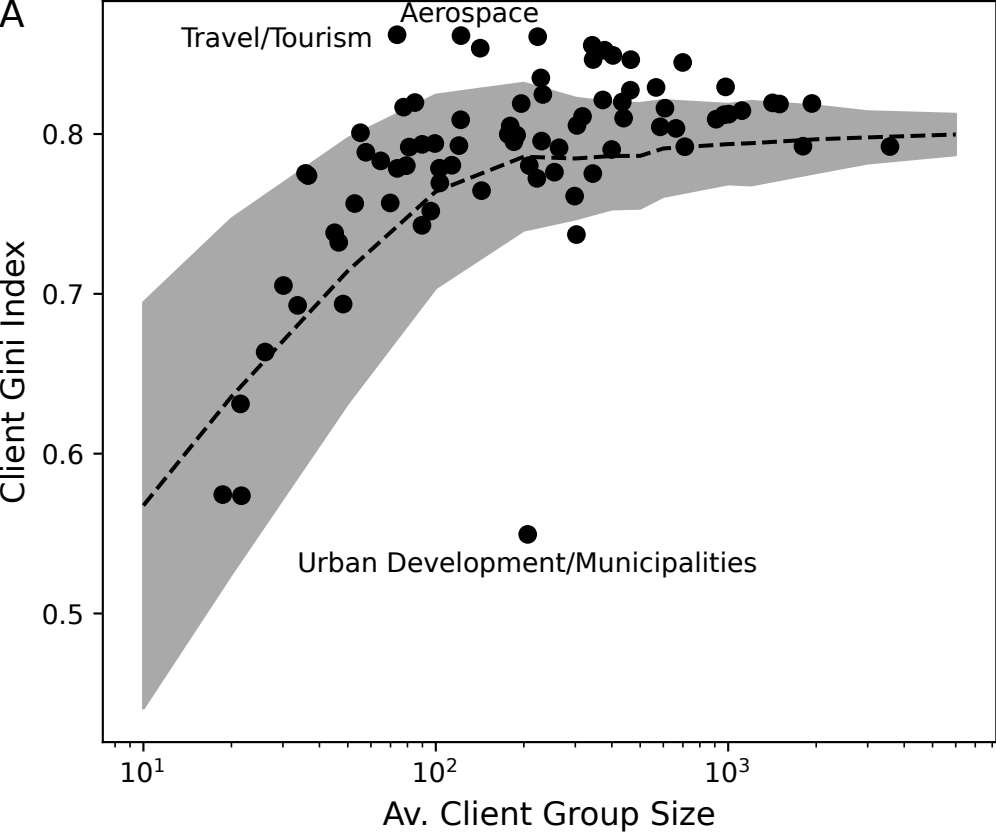

B

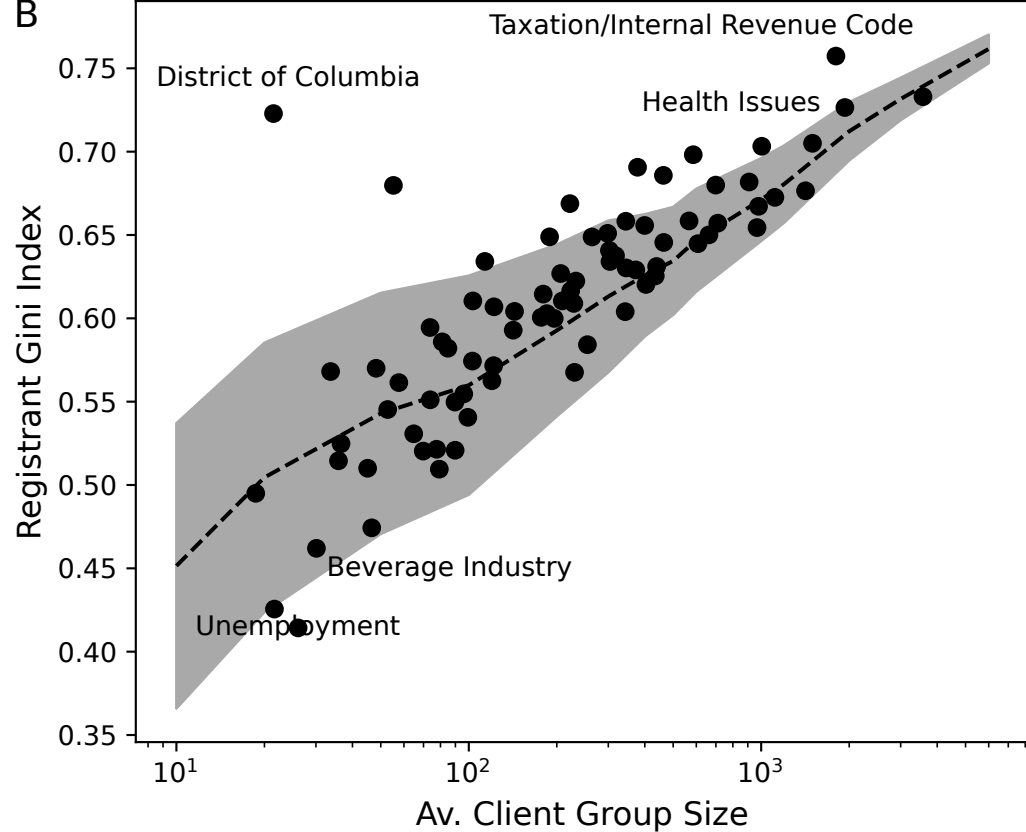

Supplement: Supplementary file 1 [file fig_sm_gini_by_issue.pdf]
